# Supplementary material for: A Qualitative Analysis Framework for mHealth Privacy Practices
Source: arXiv:2405.17971 source file (2024-05-28)
Supplement: Supplementary file 1 [file 8_appendices.tex]

\clearpage
\appendices

\onecolumn

\section{Mapping of PHI Classification Schemes}

\begin{figure}[h]
  \centering
  \includegraphics[width=.64\textwidth]{figures/data_mapping.pdf}
  \caption{Mapping of specificity and privacy labels to observed PII/PHI types. Due to a lack of fine-grained Google Play Privacy Label Subcategories for \textit{Fitness Info} and \textit{Health Info}, three supplemental subcategories are added to accurately reflect the observed PHI categories.}
  \label{fig:hoststats}
\end{figure}

\clearpage

\section{Synthetic Persona}
\label{app:persona}
